# Supplementary material for: RGB-Event ISP: The Dataset and Benchmark
Source: arXiv:2501.19129 source file (2025-01-31)
Supplement: Supplementary file 1 [file 2-appendix.tex]

\newpage
\appendix

{\Large \textbf{Appendix / Supplemental Material}}

Due to space limitations in the main text, additional details are presented in the supplementary material. Specifically:
\begin{itemize}
    \item \textbf{Sec.~\ref{sec:pro-pri}}: We provide more information about the imaging principle, process and potential of the sensor.
    \item \textbf{Sec.~\ref{sec:more_dataset_details}}: We provide further details on dataset collection.
    \item \textbf{Sec.~\ref{sec:more_isp_details}}: We delve into more specifics about the controllable ISP.
    \item \textbf{Sec.~\ref{sec:more_benchmark_methods}}: We describe the characteristics of the methods compared in the Benchmark.
    \item \textbf{Sec.~\ref{sec:more_metrics}}: We provide more metrics of the methods compared in the Benchmark.
    \item \textbf{Sec.~\ref{sec:more_discussion}}: We discuss additional points of discussion.
\end{itemize}

\section{\added{Hybrid Sensor Imaging Process, Principles and Potential}\label{sec:pro-pri}}
\added{
This section describes the imaging process and working principles of the hybrid vision sensor (HVS) used in this paper.
The HVS combines quad Bayer pattern-based RGB imaging with event-based sensing, enabling high temporal resolution and high dynamic range. The following subsections elaborate on the Quad Bayer structure, event generation principles, and rolling shutter readout process.
}

\subsection{\added{Quad Bayer Pattern and RGB Imaging}}
\added{
The hybrid sensor utilizes a quad Bayer pattern, as shown in Fig.~\ref{fig:0-CoverFigure-Release}, where each group of four pixels consists of three color pixels (red, green, and blue) and one event pixel.
Let $I_{RAW}$ represent the RAW image captured by the sensor, with pixel intensity values denoted as $I_{RAW}(x, y)$.
For the RGB pixels, the values correspond to the photonic response of the sensor to incoming light, represented by:
\begin{equation}
I_{RGB}(x, y) = K_{RGB} \cdot \Phi(x, y) + N_{RGB},
\end{equation}
where $\Phi(x, y)$ is the incident light intensity, $K_{RGB}$ is the sensitivity coefficient, and $N_{RGB}$ is the noise term.
}

\added{
The quad Bayer pattern increases the effective resolution of the sensor by allowing demosaicing algorithms to interpolate missing color information. Additionally, the rolling shutter mechanism is used to sequentially expose rows of the sensor, resulting in temporal offsets across the frame. This is illustrated in Fig.~\ref{fig:16-aplex_time_stamps}.
}

\begin{figure}[t!]
\centering
\includegraphics[width=\linewidth]{images/R1-Motion-LowLight.pdf}
\caption{\small \added{In fast-motion scenarios and low-light conditions, real-world data demonstrates the advantages of events in achieving higher temporal resolution and greater dynamic range. For example, in the fast-motion scene, the color checker in (a) exhibits blurred edges, while the corresponding short-term event frame shows sharper edges, capturing motion more accurately. In low-light conditions, (b) illustrates the limitations of traditional RGB imaging, where details are lost due to insufficient lighting. However, as shown in (d) and (f), the event data captures motion effectively even under low light. Nevertheless, it is also evident that events exhibit increased noise levels in low-light conditions, as highlighted in (f). Our data opens the possibility for future low-light enhancement and deblurring in the RAW domain via events.}}
\label{fig:R1-Motion-LowLight}
\end{figure}

\subsection{\added{Event Generation Principles}}
\added{
In addition to RGB imaging, the hybrid sensor includes event pixels that detect changes in luminance. These event pixels operate in the logarithmic domain and generate an event $E(x, y, t, p)$ whenever the change in logarithmic intensity exceeds a predefined threshold $\theta$. The mathematical model for event generation is as follows:
\begin{equation}
\Delta L(x, y, t) = \log(I(x, y, t)) - \log(I(x, y, t - \Delta t)),
\end{equation}
\begin{equation}
E(x, y, t, p) =
\begin{cases}
1, & \text{if } \Delta L(x, y, t) > \theta, \\
-1, & \text{if } \Delta L(x, y, t) < -\theta,
\end{cases}
\end{equation}
where $I(x, y, t)$ is the light intensity at pixel $(x, y)$ and time $t$, $\Delta t$ is the sampling interval, and $p \in \{-1, 1\}$ represents the polarity of the event (indicating an increase or decrease in luminance)
}

\added{\textbf{High Temporal Resolution:}
The event generation process is asynchronous and occurs independently at each pixel, triggered only when a significant luminance change is detected. This enables extremely high temporal resolution, as events can be recorded at microsecond-scale intervals. Let $f_{temporal}$ represent the temporal resolution of event recording, which depends on the sampling interval $\Delta t$:
\begin{equation}
f_{temporal} = \frac{1}{\Delta t}.
\end{equation}
This high temporal resolution allows the sensor to effectively capture rapid motion and high-speed dynamics that traditional RGB cameras, limited by frame rates, cannot resolve. For example, a rolling ball or moving object creates a continuous stream of events corresponding to pixel-level luminance changes, enabling precise tracking of motion trajectories in real-time. This characteristic is particularly advantageous for motion deblurring and temporal interpolation tasks.
}

\added{
\textbf{High Dynamic Range (HDR):}
The logarithmic domain operation of the event pixels inherently provides a high dynamic range. Unlike traditional RGB sensors, which saturate under bright lighting conditions or lose detail in shadows, event pixels respond to relative changes in luminance rather than absolute intensity. Let $I_{max}$ and $I_{min}$ represent the maximum and minimum detectable intensities, respectively. The dynamic range $DR$ can be expressed in decibels (dB) as:
\begin{equation}
DR = 20 \log_{10} \left(\frac{I_{max}}{I_{min}}\right).
\end{equation}
Because events are triggered by logarithmic intensity changes, the sensor is capable of detecting changes over a wide range of luminance levels, from very dark to extremely bright conditions. This property enables effective operation in scenarios with challenging lighting conditions, such as low-light environments or scenes with high contrast between bright and shadowed regions.
}

\added{
\textbf{Practical Implications:}
The combination of high temporal resolution and high dynamic range makes the hybrid sensor particularly well-suited for applications involving fast motion or extreme lighting conditions. As illustrated in Fig.~\ref{fig:R1-Motion-LowLight}, events accurately capture motion details even in low-light scenarios while preserving high-frequency temporal information. These unique characteristics complement the RGB output, enhancing the performance of hybrid sensor ISP tasks such as motion deblurring, HDR reconstruction, and low-light enhancement.
}

\subsection{\added{Rolling Shutter and Temporal Alignment}}
\added{
The RGB output of the hybrid sensor follows a rolling shutter exposure mechanism, as shown in Figure~\ref{fig:16-aplex_time_stamps}. In this method, each row of the sensor is exposed sequentially, introducing temporal offsets between rows. Let $t_{start}(r)$ and $t_{end}(r)$ represent the start and end times of exposure for row $r$, respectively. The effective exposure time for row $r$ is given by:
\begin{equation}
T_{exp}(r) = t_{end}(r) - t_{start}(r).
\end{equation}
}
\added{To achieve temporal alignment between the RGB and event streams, the event data are synchronized with the rolling shutter exposure times.
Both events and frames have unified timestamps to ensure time alignment.
This alignment is critical for event-guided ISP tasks, where temporal information from events complements the spatial information in RGB frames.}

\begin{figure}[t!]
\centering
\includegraphics[width=\linewidth]{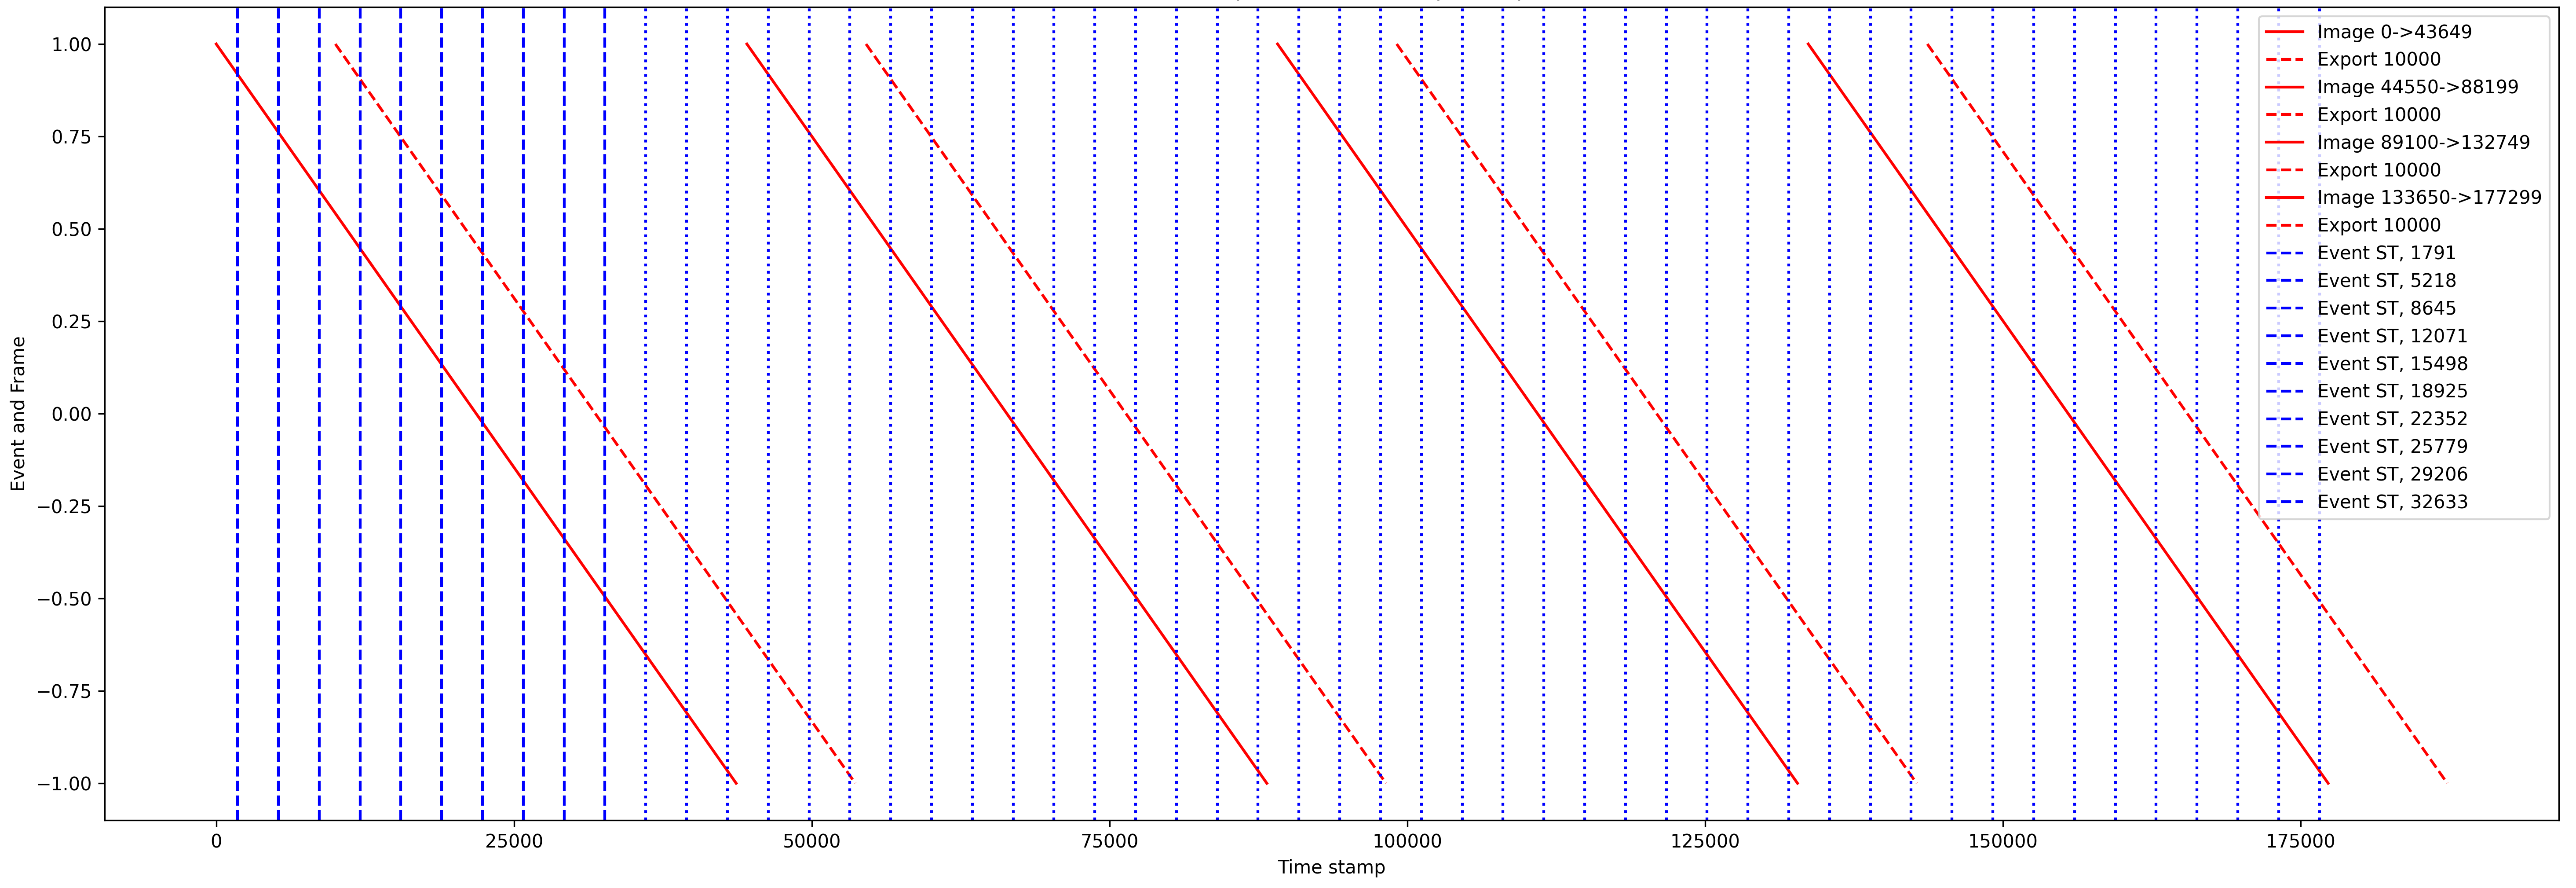}
\caption{The camera utilized for data collection features a rolling shutter mode.
The horizontal axis in the figure represents time, and the vertical axis represents each row.
Our sensor outputs both APS frames and EVS events concurrently, with both being aligned in space and time.
Specifically, the APS frames are captured using a rolling shutter exposure method.
In the diagram, the red lines represent the rolling shutter pattern; the solid red line corresponds to the start of the rolling shutter exposure, and the dashed line signifies the end of the exposure.The blue straight line represents events.}
\label{fig:16-aplex_time_stamps}
\end{figure}

\subsection{\added{Potential Benefits of Events for Different Tasks in ISP}}

\added{
\textbf{Demosaicing:}
\textit{Task Objective:} Reconstruct the full-resolution RGB image $I_{RGB}(x, y)$ from incomplete color samples in the quad Bayer pattern.
\textit{Benefits of Events:} High temporal resolution events provide precise edge information via spatial gradients $\nabla E(x, y, t)$:
\[
\nabla E(x, y, t) = \left( \frac{\partial E}{\partial x}, \frac{\partial E}{\partial y} \right),
\]
guiding interpolation along edges and reducing artifacts like color fringing. The high dynamic range aids in preserving details across varying luminance levels.
}

\added{
\textbf{Denoising:}
\textit{Task Objective:} Reduce noise $N_{RGB}$ in RAW image $I_{RAW}(x, y)$ to enhance image quality.
\textit{Benefits of Events:} Events, triggered by significant luminance changes $\Delta L(x, y, t) > \theta$, help differentiate signal from noise. By weighting the denoising process with event activity $E(x, y, t)$:
\[
I_{\text{denoised}}(x, y) = I_{RAW}(x, y) - w(x, y) \cdot N_{RGB}(x, y),
\]
where $w(x, y) = f(E(x, y, t))$, we suppress noise while preserving details in dynamic regions.
}

\added{
\textbf{White Balancing:}
\textit{Task Objective:} Adjust image colors to render neutral whites under varying illumination.
\textit{Benefits of Events:} Using event rate $r_E(x, y) = \frac{\Delta E}{\Delta t}$, we detect illumination changes and adjust white balance coefficients $K_{\text{WB}}$:
\[
I_{\text{WB}}(x, y) = K_{\text{WB}} \cdot I_{RAW}(x, y),
\]
enabling real-time adaptation to lighting variations due to the high dynamic range and temporal resolution of events.
}

\added{
\textbf{Color Correction:}
\textit{Task Objective:} Map image colors to a standard color space for accurate representation.
\textit{Benefits of Events:} Events highlight regions with significant luminance shifts, indicating potential color deviations. Incorporating event information into the color correction matrix $\mathbf{M}_{\text{CC}}(E)$:
\[
I_{\text{corrected}}(x, y) = \mathbf{M}_{\text{CC}}(E(x, y, t)) \cdot I_{\text{WB}}(x, y),
\]
allows dynamic adjustment for scene changes, enhancing color fidelity, especially in scenes with rapid motion or high contrast.
}

\added{In summary, the hybrid sensor enables simultaneous RGB and event data acquisition, leveraging the strengths of both modalities.
The RGB data provide high spatial resolution, while the event data capture motion and high-frequency changes with low latency and high dynamic range.
This unique combination not only enhances the traditional ISP process but also opens up significant potential for advanced imaging applications.
This combination facilitates advanced imaging tasks, including motion deblurring, and low-light enhancement in future, as show in Fig.~\ref{fig:14-MoreDatasetSamples}.}

\begin{figure}[t!]
\centering
\includegraphics[width=\linewidth]{images/R5-ImageWithEvents.pdf}
\caption{\small \added{More samples in our dataset, from left to right: RAW, Good RGB frame and corresponding events..}}
\label{fig:R5-ImageWithEvents}
\end{figure}

\section{More Details about Dataset Collection\label{sec:more_dataset_details}}

\added{In Fig.~\ref{fig:R5-ImageWithEvents}, we present additional samples from our dataset, showcasing the diversity and richness of the collected data. The figure includes examples of RAW images, their corresponding high-quality RGB frames, and the associated event streams. These examples highlight the variety of scenes captured, encompassing urban environments with buildings, natural landscapes with vegetation, intricate textures, vibrant flowers, and more.}

\added{
To ensure accurate color representation, each scene includes an image featuring a color card, which is systematically used for color calibration and estimation during the dataset processing. This approach enhances the reliability and usability of the dataset for ISP tasks.
}

In Fig.~\ref{fig:14-MoreDatasetSamples}, we present additional data collection scenarios, encompassing various scenes and different weather conditions.
We used LabelMe~\citep{russell2008labelme} to annotate the positions of the ColorChecker, specifically marking four points: cyan, white, brown, and black. Fig.~\ref{fig:15-LabelMe} shows our annotation interface.
All annotated location information is stored in JSON format and forms a one-to-one correspondence with the image.

\added{
\begin{table}[!ht]
\centering
\caption{Size Comparison of Related Datasets. The resolution of MIPI datasets is not uniform. \label{tab:dataset_comparison}}
\resizebox{1\linewidth}{!}{
\setlength{\tabcolsep}{0.027\linewidth}{
\begin{tabular}{lcrcccr}
\hline
\textbf{Dataset} & \textbf{Resolution} & \textbf{Scale} & \textbf{Real-World} & \textbf{Events} & \textbf{Tasks} & \textbf{Publication} \\ \hline
Ours & $2248 \times 3264$ & 3373 & Yes & Yes & Hybrid Sensor ISP & - \\

MIPI & $2040 \times 1356$ & 800 & No & No & Hybrid Sensor ISP & CVPR 2024 \\ \hline

ISPW & $1368 \times 1824$ & 197 & Yes & No& ISP & ECCV 2022 \\
NR2R & $3464\times 5202$ & 150 & Yes & No & ISP & CVPR 2022 \\
DeepISP & $3024\times 4032$ & 110 & Yes & No & ISP & IEEE TIP 2018 \\ \hline
\end{tabular}
}}
\end{table}
}

\subsection{Discussion on Dataset Diversity}

\added{By including diverse real-world scenarios, our dataset provides a robust foundation for training and benchmarking Event-ISP algorithms.
To better demonstrate the diversity of the image content of our dataset, we apply ChatGPT-4o to generate a detailed caption for each video and summarize the key elements, lighting conditions, and texture details in the dataset.
The scene and object lighting in the dataset are also summarized by ChatGPT, as shown in the Fig.~\ref{fig:R6-ChatGPT-Object}.
The conversation with ChatGPT is shown in Fig.~\ref{fig:18-ImageCaption-1}.
The summarized key elements, lighting conditions, atmosphere, and other observations across all images are:}

\added{
\begin{itemize}
    \item \textbf{Key Elements:}
    \begin{itemize}
        \item \textbf{\textit{(1) Architecture and Urban Design:}} Modern multi-story buildings; reflective glass panels; paved open areas; streetlights, and signs.
        \item \textbf{\textit{(2) Landscaping and Natural Elements:}} Landscape greenery including trees, shrubs, and grass; specific plants and flowers; wet surfaces in rain.
        \item \textbf{\textit{(3) Objects and Tools:}} Everyday items like fruits on a table and hydrant-like structures with signs; workspace equipment and office tools.
    \end{itemize}
    \item \textbf{Lighting Conditions:}
    \begin{itemize}
        \item \textbf{\textit{(4) Natural Light:}} Most outdoor scenes feature skies, providing diffused, soft natural lighting, either in bright or dim scenarios.
        \item \textbf{\textit{(5) Artificial Light:}} Indoor scenes utilize artificial lighting, resulting in muted tones and soft shadows.
        \item \textbf{\textit{(6) Reflections and Textures:}} Wet surfaces and glossy materials in outdoor images amplify reflective textures and subtle lighting nuances.
    \end{itemize}
    \item \textbf{Other Observations:}
    \begin{itemize}
        \item \textbf{\textit{(7) Attention to Detail:}} Fine textures, like foliage, building surfaces, and small objects.
        \item \textbf{\textit{(8) Balanced Composition:}} Images consist of balanced structured urban elements with natural greenery.
    \end{itemize}
\end{itemize}
}

\begin{figure}
    \centering
    \includegraphics[width=0.6\linewidth]{images/R6-ChatGPT-Object.png}
    \caption{\added{Use ChatGPT to identify the main scenes in the dataset and count their proportions.}}
    \label{fig:R6-ChatGPT-Object}
\end{figure}

\subsection{Discussion on Dataset Scale}

\added{To further demonstrate the adequacy of our dataset, we provide a comparative analysis with the most related datasets in Table~\ref{tab:dataset_comparison}. Our dataset contains 3,373 images with a resolution of $2248 \times 3264$ pixels (approximately 7.3 million pixels per image). Compared to MIPI, which includes only 800 images with resolutions around $2K$ (e.g., $2040 \times 1356$), our dataset is over four times larger and is based on real-world data rather than simulated data. This difference makes our dataset more representative and applicable for real-world ISP tasks.}

\added{It is worth noting that the MIPI dataset, despite its smaller scale, has already been demonstrated to support the training of large networks such as Transformers~\citep{xu2024demosaicformer}. Therefore, our larger dataset is even better suited for training and testing ISP models, offering greater potential for comprehensive research.}

\added{In addition to MIPI, we also consider prior ISP datasets such as ISPW~\citep{shekhar2022transform}, which contains 197 groups of images, some of which have higher resolutions (e.g., $4480 \times 6720$).
NR2R~\citep{li2022rendering} and DeepISP~\citep{schwartz2018deepisp} as traditional ISP datasets have no more than 200 images for training. But both have high resolution.
However, the total image count in ISPW is significantly smaller than our dataset, and it does not incorporate event data.}

\added{The scale of our dataset not only ensures a sufficient number of samples but also provides high-resolution data, enabling effective training and testing for ISP tasks. Additionally, the dataset includes diverse scenes, lighting conditions, and event streams, which further enhance its applicability to hybrid sensor ISP research.}

\added{In summary, our dataset provides a comprehensive resource for ISP research. Its real-world nature distinguishes it from existing datasets and makes it particularly well-suited for event-guided ISP tasks. Moreover, we are committed to the long-term maintenance of this dataset and plan to expand it in the future to accommodate larger and more complex tasks.}

\begin{figure}[t!]
\centering
\includegraphics[width=\linewidth]{images/R4-MoreDatasetExample.pdf}
\caption{\small \added{More dataset scenes and labels. Our dataset encompasses various indoor and outdoor scenes, captured under different weather conditions, including cloudy and sunny days. The initial segments of our videos include a ColorChecker, which has been annotated using LabelMe~\citep{russell2008labelme}.}}
\label{fig:14-MoreDatasetSamples}
\end{figure}

\begin{figure}
    \centering
    \includegraphics[width=\linewidth]{images/R6-ChatGPT.pdf}
    \caption{Describe the frames and generate a summary using ChatGPT.}
    \label{fig:18-ImageCaption-1}
\end{figure}

\begin{figure}[t!]
\centering
\includegraphics[width=0.4\linewidth]{images/15-LabelMe.png}
\caption{\small LabelMe annotation interface: We use LabelMe software to mark the four corners of a color card in images, which are white, cyan, brown, and black respectively. In practice, the images annotated by LabelMe are demosaiced from RAW format. While annotators can distinguish the colors, there are deviations in the image's inherent color representation.}
\label{fig:15-LabelMe}
\end{figure}

\begin{figure}[t!]
    \centering
    \includegraphics[width=\linewidth]{images/7-color_intensity_distribution_time.pdf}
    \caption{The distribution of colors on the color card in different frames under the same light source.}
    \label{fig:7-color_intensity_distribution_time}
\end{figure}

\section{More Details about Controllable ISP\label{sec:more_isp_details}}

The MATLAB demo  code of the Controllable ISP is provided in the end of the appendix.
In this section, we will elucidate further details in comment.

\textbf{Fixed Pattern Noise:} Practically, we capture pure black images (with the lens cap on) using different exposure times. The black frames captured with identical exposure times are averaged to obtain the fixed pattern noise. This noise indicates the potential deviations of some pixels, deviations which, if not addressed, can be exacerbated.
The physical meaning of this noise is that even without optics, these pixels will have intensity output due to dark current.

\textbf{Sensor Value Range:} Typically in the hardware design of sensors, the green channel will obtain a larger value than the red and blue channels, as shown in Fig.~\ref{fig:7-color_intensity_distribution_time}. Therefore, when capturing a cloudy sky (which appears white to the human eye), the green channel may reach its maximum value due to overexposure, while the red and blue channels do not, resulting in a pinkish hue in the sky. In such cases, we artificially set the overexposure. The specific operation is to use $95\

\section{More Details about Benchmark Methods\label{sec:more_benchmark_methods}}
In this section we explain in more detail the methods of the benchmark in the main paper.

\textbf{(1) Full Pipeline ISP} employs CNN architectures to streamline traditional ISP processes such as demosaicing, white balancing, and denoising, enabling a direct conversion from RAW images to RGB outputs in an end-to-end manner. This innovative approach has catalyzed extensive research, leading to the development of sophisticated models such as ReconfigISP \citep{yu2021reconfigisp}, Merging-ISP \citep{chaudhari2021merging}, PyNet \citep{ignatov2020replacing}, PyNetCA \citep{kim2020pynet}, InvertISP \citep{xing2021invertible}, and MV-ISPNet \citep{ignatov2020aim}. In our benchmark, we selected several models from a reputable open-source paper for comprehensive evaluation. Specifically, we chose MV-ISPNet, which secured first place at AIM 2020, demonstrating its robustness. Alongside, we included PyNet and its enhanced variant, PyNetCA, which incorporates attention layers for more in-depth analysis. Additionally, we incorporated InvertISP, known for its proven ability to adeptly handle various scenarios.

\textbf{InvertISP~\citep{xing2021invertible}:} InvertISP is a pipeline with a specially designed reversible structure for both rendering RGB images from RAW and to inversely recover the RAW data from RGB images. It uses a series of reversible affine coupling layers and $1\times 1$ convolutional layers to build a single reversible neural network that can map from RAW data to sRGB data, and can inversely restore RAW data from compressed RGB images.

\textbf{MV-ISPNet~\citep{ignatov2020aim}:} MV-ISPNet is a multi-level wavelet ISP network based on U-Net. It takes advantage of the Multi-level Wavelet CNN (MWCNN) and Residual Channel Attention Network (RCAN) architectures, minimizes information loss through residual groups and discrete wavelet transforms, and combines multiple loss functions and self-integration methods to improve image quality.

\textbf{PyNet~\citep{ignatov2020replacing}:} PyNet utilizes a stack of CNN layers with different resolution level to process the image, which allows the network to learn a more diverse set of features, ranging from global brightness / color to local texture enhancement.

\textbf{PyNetCA~\citep{kim2020pynet}:} PyNetCA is an enhanced version of the original PyNet. It adopts an inverted pyramid structure and considers both global and local features of the image through multi-scale feature fusion and residual connection. With a channel attention module (CA) to emphasize important channel features, and uses a sub-pixel reconstruction module (SRM) in the last layer to improve upsampling efficiency and image quality through $1\times 1$ convolution and sub-pixel shuffling technology.

\textbf{(2) Stage-wise ISPs:}.Instead of replacing the entire ISP pipeline with a single neural network, stage-wise learning based ISPs employ multiple specifically designed modules to perform different sub tasks and organize them sequentially or in parallel order to generate the final output. Note that these modules are sometimes trained independently in some models, in our experiment we only keep the model structures and train them end-to-end.

\textbf{CameraNet~\citep{liang2021cameranet}:} CameraNet designs two sequential modules and trains them separately to perform different tasks. The Restore-Net component is trained for demosaicing, white balancing and denoising while the Enhance-Net for sRGB gamma mapping and detail adjustments. The Pytorch version of CameraNet is not available, and therefore we experiments on a converted version.

\textbf{AWNet~\citep{dai2020awnet}:} AWNet employs two parallel UNet-based modules to capture global and local content. The modules take in the original RAW image and a pseudo-demosaiced image generated from the RAW image, then the output of these two modules are averaged to produce the final output.

\textbf{(3) Image Enhancement Network Based ISPs:}. Transformer-based models have demonstrated high capabilities in image enhancement tasks (e.g., deblurring, super-resolution). Even though these models are not specifically designed for ISP, a minor conversion (i.e. replacing the projector in the output layer) could evoke their potentials in ISP tasks.

\textbf{UNet~\citep{ronneberger2015u}:} UNet is a CNN-based model which has been widely adopted in areas of image processing due to its high performance in dealing with various sizes of images and modelling complex structures within them. In our experiment a UNet is trained to perform the task of ISP.

\textbf{Swin Transformer~\citep{lu2024event}:} Swin Transformer is a transformer based general-purpose backbone for image processing. It produces a hierarchical representation with shifted windows transformer blocks and brings greater efficiency by limiting self-attention computation to non-overlapping local windows while also allowing for cross-window connection.

\section{Benchmarking Metrics\label{sec:more_metrics}}

In addition to PSNR and SSIM, the inclusion of Natural Image Quality Evaluator (NIQE) \citep{zhang2015feature} and Perceptual Index (PI) \citep{zhang2014vsi} provides deeper insights into the perceptual quality and naturalness of images across various models, as shown in Table.~\ref{table:method_indoor_NIQE_performance}, and Table.~\ref{table:method_outdoor_NIQE_performance}.
The ablation study analysis of the methods in these two tables, including a discussion of the best performances, a comparison between event-based methods (eSL and EV-UNet) and pure RGB methods, and the differences of these methods in indoor and outdoor scenes.

\textbf{Best Performance Analysis:} \textbf{\textit{Indoor Scenes (Table.~\ref{table:method_indoor_NIQE_performance})}}: Swin-Transformer exhibited excellent performance in indoor scenes, achieving the lowest average NIQE (7.7104) and PI (7.2125) values. This indicates its advantage in enhancing both image quality and perceptual quality.
InvertISP closely followed, with an average NIQE of 8.8646 and PI of 7.8543, demonstrating good natural image quality.
AWNet also showed balanced performance, with an average NIQE of 8.5311 and PI of 7.9843.
\textbf{\textit{Outdoor Scenes (Table \ref{table:method_outdoor_NIQE_performance}.)}}:
InvertISP performed the best in outdoor scenes, achieving the lowest average NIQE (6.7187) and a relatively low PI (6.8720), especially excelling in complex flower and building scenes.
Swin-Transformer also demonstrated excellent performance in outdoor scenes, with an average NIQE of 7.0284 and PI of 7.2255.
eSL performed well in outdoor scenes, achieving an average NIQE of 6.9509 and PI of 7.1445.

\textbf{Comparison Between Event-Based Methods and Pure RGB Methods:}
eSL achieved good NIQE and PI values in both indoor and outdoor scenes. In particular, in outdoor scenes, it obtained an average NIQE of 6.9509 and PI of 7.1445, which are close to the best performances.
EV-UNet's performance was relatively average in both types of scenes. It had an average indoor NIQE of 10.6250 and PI of 9.2131; in outdoor scenes, it achieved an average NIQE of 8.2537 and PI of 7.8705.
Pure RGB Methods
Swin-Transformer, as a pure RGB method, performed excellently in both indoor and outdoor scenes. This indicates its good generalization ability when handling different scenes.
InvertISP, although a pure RGB method, performed outstandingly in outdoor scenes, especially in improving image quality under complex lighting conditions.
The event-based method eSL's performance in outdoor scenes was close to the best, which may be due to the advantage of event data in capturing dynamic and high dynamic range scenes.
EV-UNet's performance was slightly inferior to eSL, which may be related to its model structure or the degree to which it utilizes event data.
Pure RGB methods like Swin-Transformer and InvertISP performed outstandingly, indicating that even without event data, excellent performance can be achieved through improved model structures and algorithms.

\textbf{Differences Between Indoor and Outdoor Scenes:}
Performance Differences: Most methods exhibit better NIQE and PI values in outdoor scenes than in indoor scenes. This may be because outdoor scenes have more complex lighting conditions and content, providing more information to the models.
Advantages of Event-Based Methods: Event-based methods display more significant advantages in outdoor scenes, especially when handling rapid changes and high dynamic range environments. In such cases, event data can provide additional information to improve image quality.
Model Generalization Ability: Models like Swin-Transformer maintain consistently high performance in both indoor and outdoor scenes, demonstrating good generalization ability suitable for various environments.

\added{
\textbf{Impact of Hyperparameters on the Model:}
We observed that hyperparameters can have a impact on model performance. For instance, adjustments to learning rate, batch size, or the choice of optimizer often lead to measurable variations in results. As a benchmark study, we strive to ensure fair and unbiased evaluation across all methods by carefully tuning hyperparameters to achieve reasonable performance. However, finding the optimal hyperparameters for each model remains a challenging task, particularly given the computational costs and the inherent differences in how models respond to tuning.
In practice, hyperparameter tuning often requires balancing empirical results with theoretical insights, as exhaustive grid searches are rarely feasible.
Despite these challenges, we will provide all training codes to ensure transparency and reproducibility, while acknowledging that further fine-tuning might yield even better results for some models.
}

In summary, the best-performing models vary across different scenes; however, Swin-Transformer and InvertISP demonstrate excellent performance in both indoor and outdoor environments.
The event-based method eSL performs close to the best in outdoor scenes, confirming the effectiveness of event data in complex scenes.
Pure RGB methods can also achieve excellent performance by improving model structures. However, in specific scenes, the introduction of event data may provide additional advantages.
The performance differences of methods in indoor and outdoor scenes suggest that model design and training need to consider scene characteristics to achieve the best results.

\begin{table}[t!]
\centering
\caption{Comparison of Methods on HVS ISP Dataset indoor scenes. $^*$ refer to the results obtained by the same model with different hyperparameters.}

\resizebox{1\linewidth}{!}{
\setlength{\tabcolsep}{0.012\linewidth}{
\begin{tabular}{lrrrrrrrrrrrr}
\toprule
&
\multicolumn{2}{c}{\texttt{1-In-Fruit-2}}
&
\multicolumn{2}{c}{\texttt{3-In-ColChecker-40}}
&
\multicolumn{2}{c}{\texttt{4-In-RLChart-10}}
&
\multicolumn{2}{c}{\texttt{Average}} \\
\textbf{Methods}
& \textbf{NIQE}  & \textbf{PI}
& \textbf{NIQE}  & \textbf{PI}
& \textbf{NIQE}  & \textbf{PI}
& \textbf{NIQE}  & \textbf{PI} \\
\midrule
\textbf{PyNET}
& 10.5604 & 8.9322 & 8.6510 & 7.8808 & 8.6960 & 7.9034 & 9.3024 & 8.2388 \\
\textbf{PyNET$^*$}
& 10.6142 & 9.0591 & 9.5254 & 8.4616 & 9.2743 & 8.2574 & 9.8046 & 8.5927 \\
\textbf{PyNetCA}
& 9.5175  & 8.4227 & 9.5633 & 8.3391 & 10.0280 & 8.4848 & 9.7029 & 8.4155 \\
\textbf{InvertISP}
& 9.6301  & 8.2957 & 7.7260 & 7.2639 & 9.2377  & 8.0033 & 8.8646 & 7.8543 \\
\textbf{MV-ISPNet}
& 10.8919 & 9.2025 & 9.6756 & 8.3477 & 9.3904  & 8.3674 & 9.9859 & 8.6392 \\
\textbf{CameraNet}
& 771.8745 & 392.2881 & 771.8748 & 392.2880 & 771.8735 & 392.2873 & 771.8743 & 392.2878 \\
\textbf{CameraNet$^*$}
& 667.3576 & 335.3488 & 667.356 & 335.3535 & 667.3693 & 335.3525 & 667.3644 & 335.3501 \\
\textbf{AWNet}
& 9.0410  & 8.4831 & 8.8963 & 8.2489 & 7.6562  & 7.2208 & 8.5311 & 7.9843 \\
\textbf{Swin-Transformer}
& 7.8467  & 7.3106 & 7.9101  & 7.2932 & 7.3744 & 7.0336 & 7.7104 & 7.2125 \\
\textbf{UNet}
 & 10.7405 & 9.3207 & 9.7168  & 8.6760 & 9.5778 & 8.5257 & 10.0117 & 8.8408 \\
\textbf{UNet$^*$}
& 11.5525 & 9.9720 & 10.3320 & 9.0237 & 10.7163 & 9.2440 & 10.8669 & 9.4132 \\
\hline
\textbf{eSL}
& 8.9799  & 8.1130 & 8.5955  & 7.8486 & 8.9683  & 8.0099 & 8.8479  & 7.9905 \\
\textbf{EV-UNet}
& 10.3218 & 9.2965 & 10.7447 & 9.1840 & 10.8084 & 9.1588 & 10.6250 & 9.2131 \\

\toprule
\label{table:method_indoor_NIQE_performance}
\end{tabular}
}}

\end{table}

\begin{table}[t!]
\centering
\caption{Comparison of methods on HVS ISP dataset outdoor scenes. $^*$ refer to the results obtained by the same model with different hyperparameters.}

\resizebox{1\linewidth}{!}{
\setlength{\tabcolsep}{0.012\linewidth}{
\begin{tabular}{lrrrrrrrrrrrr}
\toprule
&
\multicolumn{2}{c}{\texttt{2-OUT-Tree-2}}
&
\multicolumn{2}{c}{\texttt{3-Out-Flower-2}}
&
\multicolumn{2}{c}{\texttt{4-Out-Building-1}}
&
\multicolumn{2}{c}{\texttt{Average}} \\
\textbf{Methods}
& \textbf{NIQE}  & \textbf{PI}
& \textbf{NIQE}  & \textbf{PI}
& \textbf{NIQE}  & \textbf{PI}
& \textbf{NIQE}  & \textbf{PI} \\
\midrule
\textbf{PyNET}
& 8.9608 & 8.2063 & 8.4138 & 7.8977 & 8.0532 & 7.6866 & 8.4759 & 7.9302 \\
\textbf{PyNET$^*$}
& 9.3716 & 8.4749 & 9.2355 & 8.2926 & 9.1500 & 8.2384 & 9.2523 & 8.3353 \\
\textbf{PyNetCA}
& 8.4343 & 7.8880 & 7.9795 & 7.6717 & 7.8525 & 7.6036 & 8.0888 & 7.7211 \\
\textbf{InvertISP}
& 7.5380 & 7.3978 & 6.7139 & 6.9881 & 5.9043 & 6.2299 & 6.7187 & 6.8720 \\
\textbf{MV-ISPNet}
& 8.1110 & 7.8820 & 7.4862 & 7.2422 & 7.4597 & 7.1434 & 7.6856 & 7.4225 \\
\textbf{CameraNet}
& 771.8750 & 392.2857 & 771.8755 & 392.2860 & 771.8743 & 392.2864 & 771.8749 & 392.2860 \\
\textbf{CameraNet$^*$}
& 667.3654 & 335.3526 & 337.3615 & 335.3509 & 667.3656 & 335.3555 & 667.3632 & 335.3525 \\
\textbf{AWNet}
& 8.6385 & 8.3241 & 8.4038 & 8.1231 & 7.0224 & 7.4135 & 8.0216 & 7.9536 \\
\textbf{Swin-Transformer}
& 7.4143 & 7.4885 & 7.2316 & 7.4287 & 6.4391 & 6.7594 & 7.0284 & 7.2255 \\
\textbf{UNet}
& 8.8706 & 8.2537 & 8.2972 & 7.8604 & 8.2363 & 7.7737 & 8.4680 & 7.9626 \\
\textbf{UNet$^*$}
& 8.8747 & 8.2149 & 8.4267 & 7.9218 & 8.4236 & 8.0117 & 8.5750 & 8.0495 \\
\hline
\textbf{eSL}
& 7.8569 & 7.7214 & 6.7929 & 7.0928 & 6.2029 & 6.6194 & 6.9509 & 7.1445 \\
\textbf{EV-UNet}
& 8.5472 & 8.0862 & 8.1830 & 7.8198 & 8.0310 & 7.7055 & 8.2537 & 7.8705 \\

\toprule
\label{table:method_outdoor_NIQE_performance}
\end{tabular}
}}

\end{table}

\section{More Discussion\label{sec:more_discussion}}

\begin{figure}
    \centering
    \includegraphics[width=\linewidth]{images/18-indoor-outdoor.pdf}
    \caption{Event counts in indoor and outdoor scenes. We randomly selected an indoor scene and an outdoor scene. The indoor scene has a strong periodic change, while the outdoor scene does not have a strong periodic change.}
    \label{fig:18-indoor-outdoor}
\end{figure}

\textbf{Impact of Indoor Light Flicker:} As shown in Fig.~\ref{fig:18-indoor-outdoor}, indoor light sources exhibit periodic flicker, whereas outdoor light sources do not have this distinct periodic flicker. This issue has also been noted in previous research~\citep{xu2024seeing}. Addressing this problem is crucial for enhancing image quality. There are two potential solutions: first, applying data augmentation during data input to enable the network to robustly handle flicker issues; and second, using temporal filtering techniques to mitigate the flicker problem.
\begin{figure}
    \centering
    \includegraphics[width=0.6\linewidth]{images/19-EV-UNet.pdf}
    \caption{\small EV-UNet framework.}
    \label{fig:19-EV-UNet}
\end{figure}

\textbf{Network Structure of EV-UNet:} EV-UNet integrates an event encoding branch into the existing UNet architecture, adding the results of both encoders during the decoding process. Despite this being a simple attempt, we observed that incorporating events can significantly enhance performance in outdoor scenes. For more detailed visual results, please refer to Fig.~\ref{fig:17-MoreVisualization-1} and Fig.~\ref{fig:17-MoreVisualization-2}.

\added{
\textbf{Analysis of Overall and Scene-Specific Performance:}
The results in Tab.~\ref{table:method_indoor_outdoor_performance} reveal both overall performance trends and context-specific strengths. For example, UNet demonstrates strong robustness with an \texttt{All-Average} PSNR of 29.97, performing well across diverse scenarios. Similarly, MV-ISPNet excels in outdoor scenes, but its performance drops indoors.
These findings underline the need to consider scene specific impacts when applying ISP methods, as overall metrics do not always reflect performance in individual contexts. Future research should focus on adapting ISP methods to specific scenarios to ensure optimal outcomes across diverse settings.}

\begin{table}[t]
\centering
\caption{\small Comparison of Methods on HVS ISP Dataset indoor and outdoor scenes.}
\resizebox{1\linewidth}{!}{
\setlength{\tabcolsep}{0.012\linewidth}{
\begin{tabular}{l ccc ccc ccc}
\toprule
& \multicolumn{3}{c}{\texttt{Out-Average}}
& \multicolumn{3}{c}{\texttt{In-Average}}
& \multicolumn{3}{c}{\texttt{All-Average}} \\
\textbf{Methods}
& \textbf{PSNR}$\uparrow$   & \textbf{SSIM}$\uparrow$  & $L_1$$\downarrow$
& \textbf{PSNR}$\uparrow$   & \textbf{SSIM}$\uparrow$  & $L_1$$\downarrow$
& \textbf{PSNR}$\uparrow$   & \textbf{SSIM}$\uparrow$  & $L_1$$\downarrow$ \\
\midrule
\textbf{PyNET}
& 32.47 & 0.9785 & 0.0180 & 11.97 & 0.7664 & 0.2412 & 22.22 & 0.8725 & 0.1296 \\
\textbf{PyNET$^*$}
& 29.37 & 0.9652 & 0.0265 & 17.36 & 0.8437 & 0.1494 & 23.37 & 0.9044 & 0.0880 \\
\textbf{PyNetCA}
& 31.76 & 0.9762 & 0.0207 & 27.72 & 0.9431 & 0.0540 & 29.74 & 0.9596 & 0.0373 \\
\textbf{InvertISP}
& 27.59 & 0.9364 & 0.0281 & 28.27 & 0.9392 & 0.0254 & 27.93 & 0.9378 & 0.0268 \\
\textbf{MV-ISPNet}
& 29.76 & 0.9662 & 0.0232 & 31.12 & 0.9664 & 0.0207 & 30.44 & 0.9663 & 0.0219 \\
\textbf{CameraNet}
& 11.36 & 0.2618 & 0.2266 & 13.04 & 0.2591 & 0.2013 & 12.20 & 0.2605 & 0.2139 \\
\textbf{CameraNet$^*$}
& 12.30 & 0.3953 & 0.2096 & 12.68 & 0.2672 & 0.2073 & 12.49 & 0.3312 & 0.2085 \\
\textbf{AWNet}
& 17.04 & 0.9180 & 0.0879 & 27.03 & 0.9356 & 0.0567 & 22.04 & 0.9268 & 0.0723 \\
\textbf{Swin-Transformer}
& 25.24 & 0.9463 & 0.0354 & 25.80 & 0.9481 & 0.0304 & 25.52 & 0.9472 & 0.0329 \\
\textbf{UNet}
& 24.51 & 0.9634 & 0.0354 & 15.70 & 0.8913 & 0.1124 & 20.11 & 0.9274 & 0.0739 \\
\textbf{UNet$^*$}
& 28.17 & 0.9685 & 0.0265 & 31.76 & 0.9705 & 0.0188 & 29.97 & 0.9695 & 0.0226 \\
\textbf{eSL-Net}
& 23.02 & 0.9294 & 0.0473 & 26.13 & 0.9464 & 0.0381 & 24.57 & 0.9379 & 0.0427 \\
\textbf{EV-UNet}
& 30.11 & 0.9698 & 0.0225 & 26.04 & 0.9388 & 0.0640 & 28.08 & 0.9543 & 0.0432 \\
\bottomrule
\label{table:method_indoor_outdoor_performance}
\end{tabular}
}}
\end{table}

\clearpage
\begin{figure}
    \centering
    \includegraphics[width=\linewidth]{images/17-MoreVisualization-1.pdf}
    \caption{More visualization results.}
    \label{fig:17-MoreVisualization-1}
\end{figure}

\begin{figure}
    \centering
    \includegraphics[width=\linewidth]{images/17-MoreVisualization-2.pdf}
    \caption{More visualization results.}
    \label{fig:17-MoreVisualization-2}
\end{figure}

\clearpage
\begin{lstlisting}[language=Matlab, caption=MATLAB ISP Code.]
function ans_colors = RGBE_ISP(
    raw_npz_file,
    json_file,
    has_known_colors,
    known_colors,
    gamma)
    % RGBE_ISP: ISP for RGBE data.
    % raw_npz_file: the raw data file.
    % json_file: the json file for color card.
    % has_known_colors: has known colors.
    % known_colors: the known colors.
    % gamma: gamma value.
    fprintf('RGBE_ISP:\n');
    fprintf('   raw_npz_file :%s\n', raw_npz_file);
    fprintf('   json_file    :%s\n', json_file);
    % Read the raw data for black level calibration.
    pth_blcraw = './rawdata/FixedPatternNoise.npy';
    img_blc = readNPY(pth_blcraw);
    img_blc = double(img_blc) / 242.0;
    % get the file name
    [pathstr, file_name, ext] = fileparts(raw_npz_file);
    % Read rge quad raw data.
    % 242 is the max value of the raw data. The raw data is 8bit.
    % 242 = 255 * 0.95. The 0.95 is the saturation level.
    img_quad = readNPY(raw_npz_file);
    img_quad = max(0, min(img_quad, 242));
    img_quad = double(img_quad) / 242.0;
    img_quad = img_quad - img_blc;
    % clip the value to [0, 1]
    img_quad = max(0, min(img_quad, 1));
    [height, width] = size(img_quad);
    % demosaic the quad raw data.
    % This function can be found in the following link.
    % https://www.mathworks.com/matlabcentral/fileexchange/
    % 116085-quadbayer-cfa-modified-gradient-based-demosaicing
    img_rgb = quad_bayer_demosaic_full(
        img_quad, height, width, 'grgb', 0, 0);
    if has_known_colors
        colors = known_colors;
        ans_colors = [];
    else
        vertex_pts = get_color_card_coords_from_json(json_file);
        % check the vertex_pts has 4 points
        if size(vertex_pts, 1) ~= 4
            disp('Error: vertex_pts has not 4 points');
            return;
        end
        % get the colors from the image given 4 points' location
        % The vertex_pts is the 4 points of the color card.
        [colors, coord] = checker2colors(
            img_rgb, [4, 6], 'mode', 'auto',
            'show', false, 'vertex_pts', vertex_pts);
        % save colors to file
        color_file = sprintf('%s/%s_colors.mat', pathstr, file_name);
        save(color_file, 'colors');
        % the colors will be reture value.
        ans_colors = colors
        % check NaN value in colors. if has NaN value, return.
        if any(isnan(colors))
            disp('Error: colors has NaN value');
            fprintf('raw_npz_file: %s\n', raw_npz_file);
            return;
        end
    end
    % white balance
    wb_multipliers = [
        colors(21, 2) / colors(21, 1),
        1.0,
        colors(21, 2) / colors(21, 3)];
    img_wb = img_rgb;
    img_wb(:, :, 1) = img_wb(:, :, 1) * wb_multipliers(1);
    img_wb(:, :, 3) = img_wb(:, :, 3) * wb_multipliers(3);
    img_wb = max(0, min(img_wb, 1));
    % denoise using rgb BM3D with default parameter
    randn('seed', 0);
    sigma = 25;
    [~, img_denoise] = CBM3D(1, img_wb, sigma);
    % color correction.
    % The color card colors are sRGB from 
    % the document of the color card, 
    % treated as groundtruth sRGB under D65
    srgb = [
            112, 76, 60;
            197, 145, 125;
            87, 120, 155;
            82, 106, 60;
            126, 125, 174;
            98, 187, 166;
            238, 158, 25;
            157, 188, 54;
            83, 58, 106;
            195, 79, 95;
            58, 88, 159;
            222, 118, 32;
            25, 55, 135;
            57, 146, 64;
            186, 26, 51;
            245, 205, 0;
            192, 75, 145;
            0, 127, 159;
            43, 41, 43;
            80, 80, 78;
            122, 118, 116;
            161, 157, 154;
            202, 198, 195;
            249, 242, 238;
            ];
    srgb = srgb / 255.0; %normlization
    srgb = srgb .^ 2.2;  %sRGB to linear sRGB
    colors_wb = colors .* wb_multipliers % white balance correction
    % compute the color correction matrix.
    [cam2xyz, scale, ~, ~] = ccmtrain(colors_wb, ...
        srgb, 'omitlightness', true, 'preservewhite', true, ...
        'model', 'linear3x3', 'targetcolorspace', 'sRGB', ...
        'whitepoint', whitepoint('d65'));
    % apply the color correction matrix.
    lin_srgb = apply_cmatrix(
        img_denoise * (scale * 0.9),transpose(cam2xyz));
    lin_srgb = max(0, min(lin_srgb, 1));
    % gamma correction.
    img_srgb = lin_srgb .^ gamma;
    img_srgb = max(0, min(img_srgb, 1));
    good_rgb_file = sprintf(
        '%s/%s_good_rgb.png', pathstr, file_name);
    imwrite(img_srgb, good_rgb_file);
    fprintf('DONE: %s', good_rgb_file);
end
\end{lstlisting}
